# Supplementary material for: Bloch Ferromagnetism of Composite Fermions
Source: arXiv:2008.11630 ancillary file (2020-08-26)
Supplement: Supplementary file 1 [file Supplementary_Information.pdf]

# Supplementary Materials: Bloch Ferromagnetism of Composite Fermions


Md. Shafayat Hossain,[1,†,*] Tongzhou Zhao,[2,†] Songyang Pu,[2] M. A. Mueed,[1] M. K. Ma,[1] K. A. Villegas Rosales,[1] Y. J. Chung,[1] L. N. Pfeiffer,[1] K. W. West,[1] K. W. Baldwin,[1] J. K. Jain,[2,*] M. Shayegan[1,*]

[1]Department of Electrical Engineering, Princeton University, Princeton, New Jersey 08544, USA

[2]Department of Physics, 104 Davey Lab, Pennsylvania State University, University Park, Pennsylvania 16802, USA

[†]These authors contributed equally to this work.

[*]To whom correspondence should be addressed; E-mail: shayegan@princeton.edu.


## List of Contents


**I. Spin polarization of composite fermions**

**II. Additional evidence for the partial spin polarization of composite fermions at intermediate densities**

**II.1. Resistivity at $\nu = 1/2$ as a function of density**

**II.2. Spin polarizing the composite fermions by adding an in-plane magnetic field**

**III. Temperature-dependence of composite fermion geometric resonances**

**IV. Spin polarization of zero-field electrons**

**V. Theory**

**V.1. Wavefunction of the composite fermion Fermi-sea state**

**V.2. Fixed-phase DMC method**

**V.3. Calculation of $E_p$ and $E_s$**

**V.4. Stoner model for composite fermions**

**VI. Related phenomena**

**VI.1. Bloch ferromagnetism vis-à-vis the Mermin Wagner theorem in 2D electron systems**

**VI.2. Spontaneous valley polarization in 2D systems with anisotropic effective mass**

**VI.3. Spin polarization of 2D electrons in monolayer $MoS_2$**

# I. Spin polarization of composite fermions

In this Section, we further discuss the spin polarization of composite fermions (CFs) in light of our experimental data presented in Figs. 1 and 2 of the main text. In Fig. 2b of the main text, all the CF geometric resonance (GR) traces are presented in the same panel to depict the gradual and systematic change in the GR features as a function of density. Here in Figs. S1a–c, we separate our CF GR data in three panels: $n > n_{c2}$ (Fig. S1a), $n_{c1} < n < n_{c2}$ (Fig. S1b), and $n \leq n_{c1}$ (Fig. S1c), so that the details can be seen more clearly. Furthermore, we also include a few traces taken at higher densities, see for e.g., $n = 10.16$, 7.94, and 6.88 traces (Fig. S1a). We mark the expected field positions of the $i = 1$ CF GR assuming a fully-spin-polarized CF Fermi sea for each trace. In Figs. S1a,c, where the CFs are fully spin polarized, the locations of the CF GR minima align well with the markings. In Fig. S1b, however, the locations of the CF GR minima deviate from the markings, because the CFs in $n_{c1} < n < n_{c2}$ range are only partially spin polarized.

As we discussed briefly in the main text, the spin physics of CFs arises from a competition between the Zeeman ($E_Z$) and Coulomb ($E_C$) energies. Note that the relevant magnetic field for the $E_Z$ of the CFs is the total applied magnetic field ($B$) and not the effective field ($B^*$).[S1] $E_Z$ increases linearly with $B$ while $E_C$ goes as $\sqrt{B}$. Previous studies[S2,S3] of the spin polarization

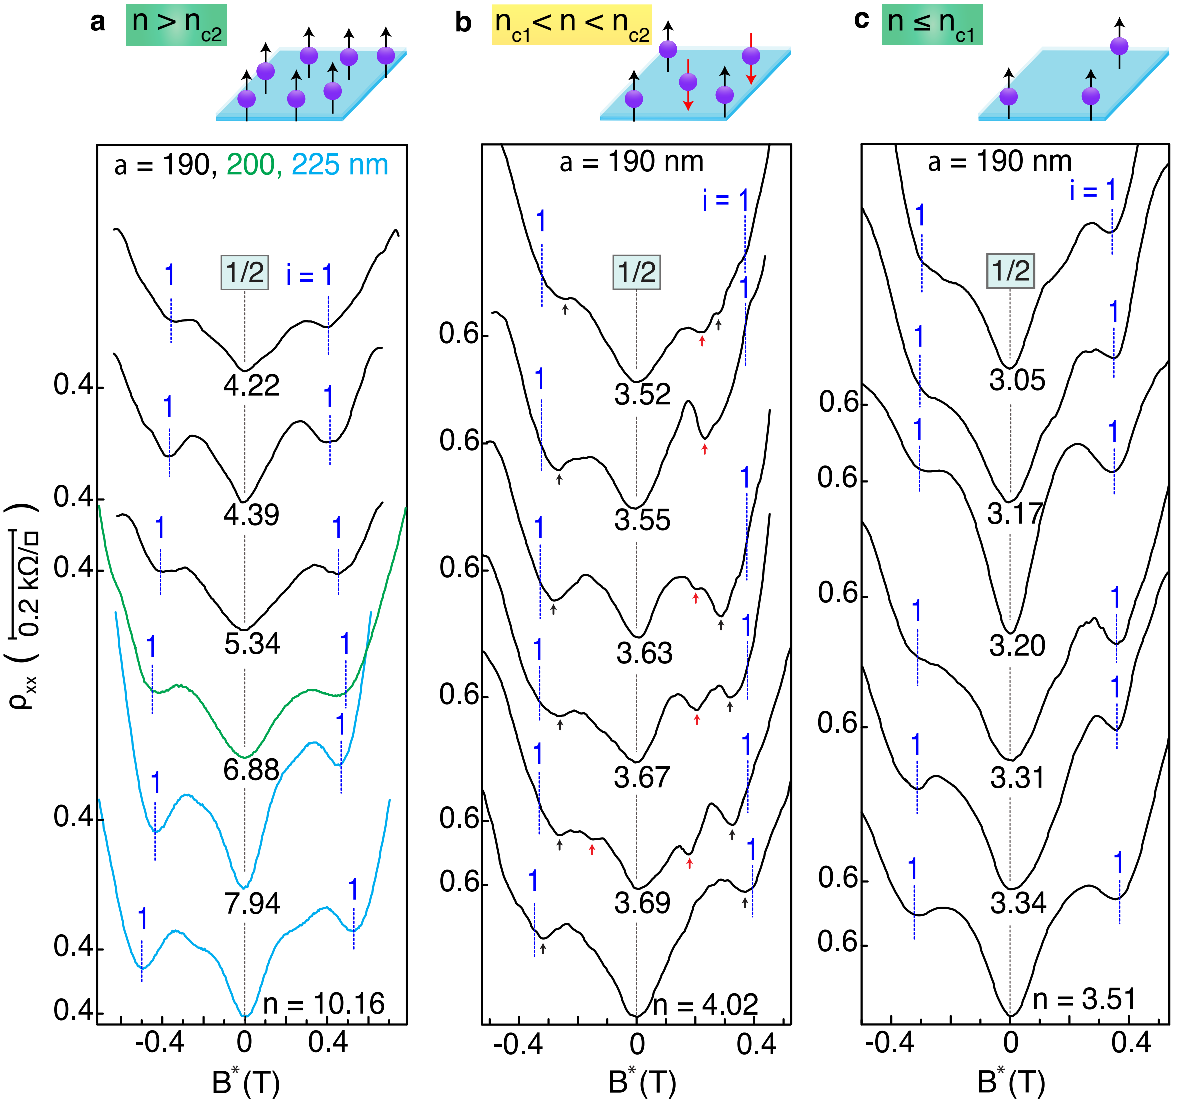


**Fig.** S1: CF GR features near $\nu = 1/2$ demonstrated by the resistance minima flanking $\nu = 1/2$ in the density ranges of: **a**, $n > n_{c2}$, **b**, $n_{c1} < n < n_{c2}$, and **c**, $n \leq n_{c1}$. The black and red arrows in panel **b** mark the positions of the minima we associate with the GR of spin-up and spin-down CFs. Vertical blue lines mark the *expected* positions for the $i = 1$ GR for fully-spin-polarized CFs.

of CFs have established that at sufficiently high electron density, when the ratio ($\alpha$) of $E_Z$ to $E_C$ exceeds a critical value ($\alpha_c \simeq 0.01$), the CFs are fully spin polarized at $\nu = 1/2$ (and other filling factors $< 1$). This is the case in the $n > n_{c2}$ region in our samples (Fig. S1a). When the

density is lowered, the ratio between $E_Z$ and $E_C$ decreases and the CFs make a transition from a fully-spin-polarized to a partially-spin-polarized phase. This is also well established in previous reports, and happens in our samples when we lower the density below $n_{c2}$ (Fig. S1b). Now, as the density is lowered even further, if the residual interaction between the CFs is ignored, one would expect spin polarization to continue to decrease. There is no reason for the CFs to become fully spin polarized again since the ratio of $E_Z$ and $E_C$ is further decreased.

What is surprising in our experiments, however, is that as we lower the density below $n_{c1}$, the CFs make a sudden transition to a fully-spin-polarized state (Fig. S1c). We attribute this transition to a Bloch-type, interaction-driven transition to a ferromagnetic state. Our detailed theoretical calculations presented in the main text and Section V of SM justify our explanation: the effective interaction strength between CFs depends on Landau level (LL) mixing, and at low densities, the CFs become more strongly interacting as the LL mixing increases. Such strong interaction between CFs then drives the system into a fully-polarized state, just as expected for a Bloch ferromagnet.

It is important to note that our experiments clearly show that both the phases above $n_{c2}$ and below $n_{c1}$ are fully spin polarized, i.e., ferromagnetic. The key point, however, is that the origin of full spin polarization is different above $n_{c2}$ and below $n_{c1}$. In light of our experiments and theoretical calculations presented in this paper, in the density range $n > n_{c2}$, the CFs are fully spin polarized because $E_Z$ dominates over the $E_C$ while below $n_{c1}$, the ferromagnetism is stabilized by inter-CF interaction. In order to discern these two ferromagnetic states, the presence of the intermediate density range $n_{c1} < n < n_{c2}$, where the CFs are partially polarized, is crucial. If the CFs did not exhibit partial spin polarization in this range, i.e., if they remained fully spin polarized at all densities, it would be impossible to infer a Bloch transition. In this context, we provide additional evidence for partial spin polarization in the range $n_{c1} < n < n_{c2}$ in the next Section (Section II).

# II. Additional evidence for the partial spin polarization of composite fermions at intermediate densities

In the main text, we provide three sets of data that support our conclusion regarding the partial spin polarization of CFs near $\nu = 1/2$ in the intermediate density regime $n_{c1} < n < n_{c2}$. First, in this density range, we observe GR minima at $|B^*_{i=1}| < 2\hbar(4\pi n)^{1/2}/ea(1 + 1/4)$; this is consistent with CFs being partially polarized (Fig. 2b and also Fig. S1b). Second, we show a resistance vs density plot (Fig. 1e of the main text) that indicates a rapid change in resistance in the density ranges, where spin-polarization changes occur. Third, in Fig. 3 of the main text, we show parallel field dependence of the CF GR features, exhibiting a transition from partial to full spin polarization in the $n_{c1} < n < n_{c2}$ range, when a sufficiently large Zeeman energy is added via applying in-plane magnetic fields, lending crucial credence to the partial spin polarization in $n_{c1} < n < n_{c2}$ at zero in-plane magnetic field.

Here we first elaborate on the origin and significance of Fig. 1e data. Next we discuss the parallel field-dependent data, a portion of which is presented in Fig. 3 of the main text. We reiterate that the presence of this intermediate density range, where the CFs are partially polarized, is very important for our conclusion.

## II.1. Resistivity at $\nu = 1/2$ as a function of density

In Fig. S2 we show the resistivity of our samples measured at $\nu = 1/2$ as a function of density. (A portion of this data is shown in Fig. 1e.) As expected, the resistivity increases when the density is lowered. There is, however, a pronounced dip in the resistivity in the density range $n_{c1} < n < n_{c2}$. This behavior is consistent with the CFs not being fully spin polarized in this density range. It is well known that 2D carrier systems have a smaller resistance when not spin polarized [see, e.g., Refs.[S4–S9]]. The origin is generally believed to be the fact that spin-unpolarized electrons are more efficient in screening the disorder potential; see e.g., Refs.[S4–S11]

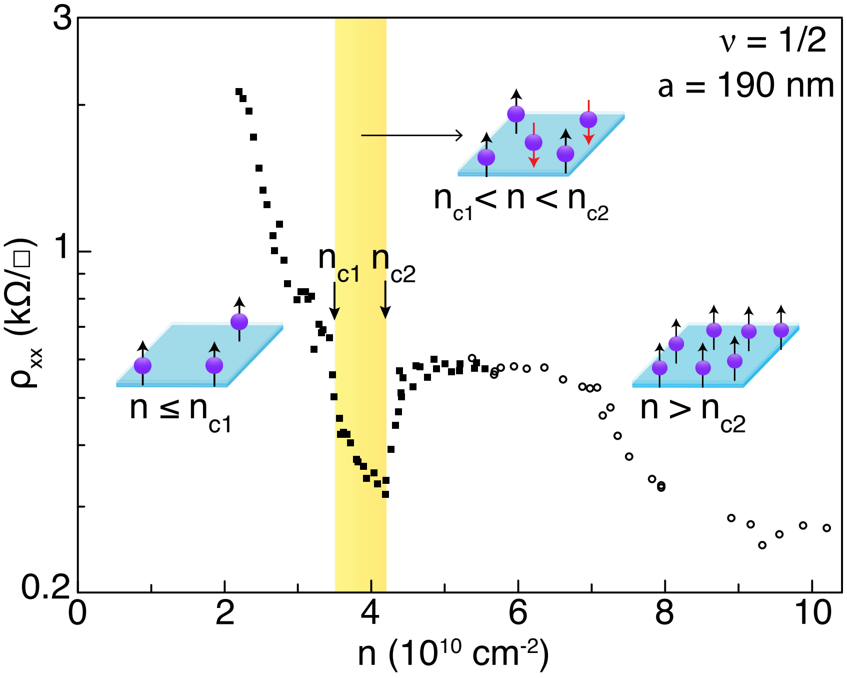


**Fig.** S2: Resistivity vs density plot for $\nu = 1/2$ CFs, revealing a decrease in $\rho_{xx}$ when the CFs are partially spin polarized. The data support our conclusion that in the ranges $n < n_{c1}$ and $n > n_{c2}$, CFs are fully spin polarized while for $n_{c2} < n < n_{c1}$, CFs are only partially spin polarized. Closed and open symbols denote the data taken from two different samples.

The CFs have also been reported to follow the same trend, with their resistance at $\nu = 1/2$ being larger when spin- (or valley-) polarized.[S12,S13] The data of Fig. S2 therefore provide further evidence that the CFs in our samples are partially spin polarized in a very small density range before making a sudden transition to a fully-magnetized state at lower densities.

## II.2. Spin polarizing the composite fermions by adding an in-plane magnetic field

In a separate set of measurements, we add a parallel (in-plane) magnetic field ($B_{||}$) by tilting the sample in the magnetic field, with $\theta$ denoting the angle between the total field direction and the normal to the 2D plane. $B_{||}$ adds to the Zeeman energy $E_Z$ while keeping the Coulomb energy $E_C$ fixed (at a given filling). In Fig. S3, we present the evolution of CF GR features as a

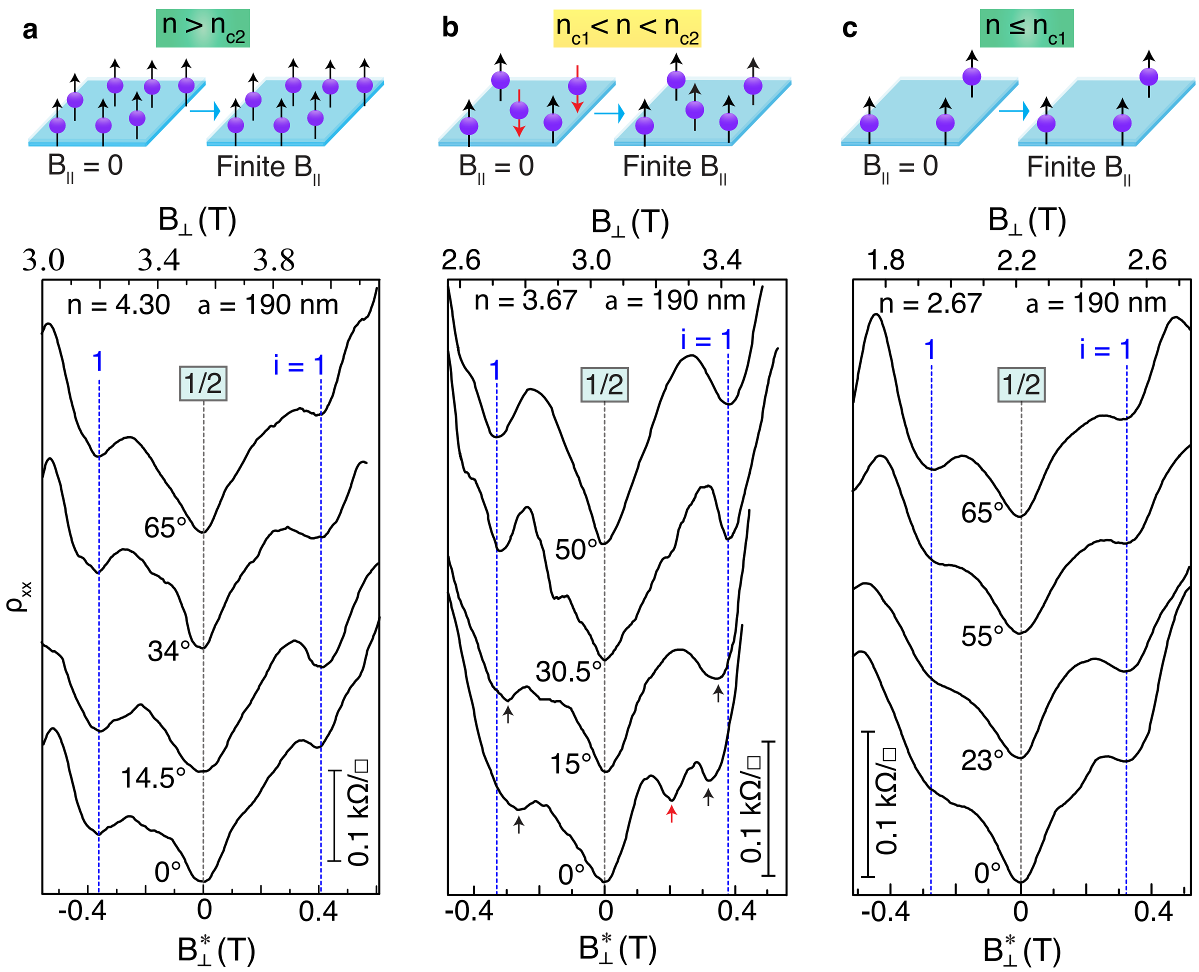


**Fig.** S3: Tilt evolution of the CF GR features near $\nu = 1/2$ for: **a**, $n = 4.30$, **b**, $n = 3.67$, and **c**, $n = 2.67$. Traces are vertically offset for clarity; the tilt angle $\theta$ is given for each trace. The *expected* positions for the $i = 1$ GRs for fully-magnetized CFs are marked with vertical blue lines. In all three panels, the scale for the applied external field $B_\perp$ is shown on top while the bottom scale is the effective magnetic field $B_\perp^*$ experienced by the CFs. The cartoons above the panels elucidate the effect of $B_{||}$.

function of $B_{||}$, similar to what is shown in Fig. 3 of the main text. Here in Fig. S3, we include additional traces at intermediate tilt angles to demonstrate the $B_{||}$-dependence of the CF GR features.

At $n = 3.67$ and $\theta = 0$, there are CFs with both $\uparrow$-spin and $\downarrow$-spin. (As in the main text, we use $10^{10}$ cm$^{-2}$ as the unit of density.) This is evident from the two $i = 1$ CF GR features on the

$B^* > 0$ side, as seen in Figs. 2b and 3b of the main text and also in Figs. S1b and S3b. When the sample is titled, however, the CFs become fully magnetized; see the upper traces in Fig. S3b where there is a clear $i = 1$ GR minimum whose position agrees very well with what is expected for fully-spin-polarized CFs. This behavior is consistent with the enhanced $E_Z$ in tilted fields favoring fully-magnetized CFs. Thus, in the $n_{c1} < n < n_{c2}$ region where the CFs are partially polarized, CFs can be forced to become fully polarized by adding additional Zeeman energy. In Fig. S3c we show tilt data for $n = 2.67$. In this low-density case, the CFs are already fully magnetized at $\theta = 0$, and show no change in their spin polarization as the sample is tilted. This trait is similar to the tilt evolution for $n > n_{c2}$, such as $n = 4.30$ (Fig. S3a), where there is no change in the position of the CF GR features, i.e., the spin polarization of the CFs, as we add in-plane magnetic fields, consistent with the CFs being fully polarized. (In some of the traces for CFs with a fully-spin-polarized Fermi sea, we observe hints of the $i = 2$ GR; examples include the trace at $\theta = 30.5^o$ in Fig. S3b, the trace at $\theta = 0^o$ in Fig. S3c, and the traces at $n =$ 10.16, 3.31, 3.17, and 3.05 in Figs. 2 and S1.) This test provides a consistency check on the partial vs. full polarization of the CFs.

# III. Temperature-dependence of composite fermion geometric resonances

Here we describe the temperature ($T$) dependence of the CF GRs. In Fig. S4 we show the CF GR features as a function of temperature over the density ranges, $n > n_{c2}$ [Fig. S4a], $n_{c1} < n < n_{c2}$ [Fig. S4b], and $n < n_{c1}$ [Fig. S4c]. In all three cases, when $T$ is increased, the GR features become weaker before disappearing at high temperatures. More importantly, however, the field positions of the GR features remain unchanged even up to the highest temperatures where we still observe GRs.

It is clear from the plots in Fig. S4 that the GR features become weaker as $T$ is raised. Such

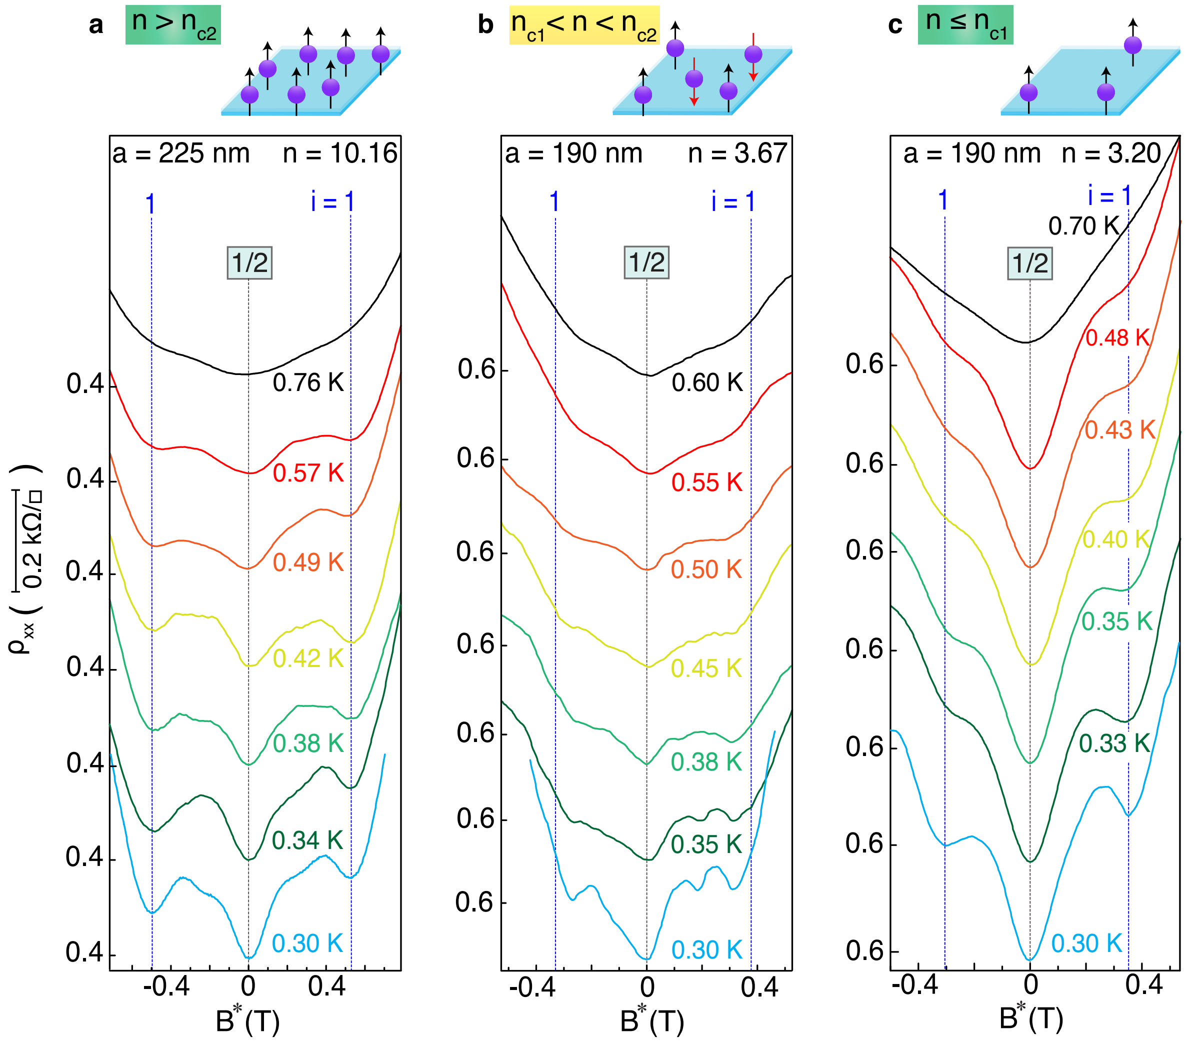


**Fig.** S4: Temperature dependence of the CF GR features for three different densities: **a**, $n = 10.16$; **b**, $n = 3.67$; and **c**, $n = 3.20$; all densities are in units of $10^{10}$ cm$^{-2}$. Theses data were taken in a separate cooldown from the data shown in the main text. In **a** and **c**, the CFs are fully spin polarized while in **b** CFs are partially spin polarized. Magneto-resistance traces are shown for seven temperatures ranging from 0.30 K to 0.76 K. Traces are vertically offset for clarity. The *expected* positions for $i = 1$ GRs, assuming fully-spin-polarized CFs, are marked with blue vertical lines.

a weakening can happen for various reasons, including: (a) The ballistic mean-free-path of the CFs can get shortened because of the extra scattering at higher temperatures. (b) At high temperatures, the thermal energy ($k_BT$) approaches the CF Fermi energy ($E_F^*$). We estimate $E_F^*/k_B$

for CFs at $\nu = 1/2$ to be 3.3, 2.0, and 1.8 K for $n = 10.16$, 3.67, and 3.20, respectively.[S14,S15] (All densities are in units of $10^{10}$ cm$^{-2}$.) Therefore, as we raise the temperature, $k_BT$ becomes a significant fraction of $E_F^*$, and can lead to the gradual weakening and the eventual disappearance of the GR features at high temperatures. (c) The CFs can also gradually lose their spin polarization as $T$ is raised; see further discussion in the next paragraph. In this case, one would expect the magnetic field positions of the GR features to move closer to $\nu = 1/2$ (similar to the GR features in the range $n_{c1} < n < n_{c2}$). However, we do not observe a measurable shift in the field positions of the GR features when the temperature is raised. Hence, we surmise that the weakening of the GR features with the rise in $T$ is linked to either the reduction of the mean-free-path of CFs or the increase in $k_BT/E_F^*$ with temperature.

Our data suggest that there is no loss of spin polarization up to the highest $T$ at which we still observe clear GR features. This might sound surprising at first sight, since it is well documented in nuclear magnetic resonance (NMR) studies that CFs tend to lose their spin polarization at high temperatures.[S14,S15] To better understand the $T$-dependence data, we compare our results to the NMR data of Melinte *et al.*,[S14] who presented data for CFs at $\nu = 1/2$ for samples with two densities $n = 14$ and 8.5. They found that the loss of spin polarization depends on $n$. For the sample with $n = 14$, there is only $5\%$ loss of polarization when $T$ is raised from 0.30 K to 0.60 K while for the sample with lower density, the loss is about $10\%$. Therefore, a reasonable estimate of the loss of spin polarization for our sample with $n = 10.16$ at $T \simeq 0.60$ K would be about $8\%$. However, at $T \gtrsim 0.57$ K, the GR minima in our samples become quite broad [Fig. S4a] and therefore such a small change in the polarization cannot be accurately detected. There is no NMR data available at very low densities ($< 8.5$) but, extrapolating the NMR to low densities, one would expect that the CFs should lose their full spin polarization more quickly as $T$ is raised. For $n = 3.20$, which is about 3 times smaller than the lowest density in NMR measurements (8.5), Fig. S4c data suggest that the GR and its position might

be anomalously robust. A possible reason for this relative robustness could be the enhanced exchange interaction between the CFs that we believe is responsible for the itinerant ferromagnetism we observe at very low densities. However, because of the very limited $T$-range where the GRs are observed, the connection between the temperature robustness and the spontaneous ferromagnetism is tenuous and requires further investigation.

# IV. Spin polarization of zero-field electrons

In this Section, we present GR data for the zero-field electrons. To draw a comparison with the CFs, similar to Fig. 1c of the main text, in Fig. S5a we plot the measured densities of a particular spin, normalized by the total electron density $n$, plotted against $n$. The plot in Fig. S5a looks simpler compared to Fig. 1c of the main text because there is no spin transition for zero-field electrons as we tune the density from $n = 10.16$ to 1.32. Therefore, we conclude that there is no Bloch ferromagnetism for zero-field electrons within the density range of this study. This is consistent with both theory and previous experiments. At $n = 1.32$, $r_s$ is only about 4.7, much smaller than the theoretically predicted value of 26 that is required to observe Bloch ferromagnetism.[S16,S17] Our data are also consistent with the results of Zhu *et al.*[S9] on GaAs two-dimensional electron systems (2DESs) which indicated a paramagnetic ground state at zero magnetic field even down to $n = 0.2$ ($r_s \simeq 12$). An intriguing aspect of our data is that the spin polarization shows a tendency to slightly increase at very low densities below $n \simeq 2$. It would be very interesting if one could lower the density even further and still observe electron GR features to probe the spin polarization at extremely low densities.

Next we briefly describe how we obtain the spin polarization for the zero-field electrons. Similar to CFs at $\nu = 1/2$, we track the GRs for the zero-field electrons. If the cyclotron orbit of the electrons becomes commensurate with the period of the applied perturbation, then a GR occurs. Quantitatively, GRs of zero-field electrons manifest at the *electrostatic* GR condition

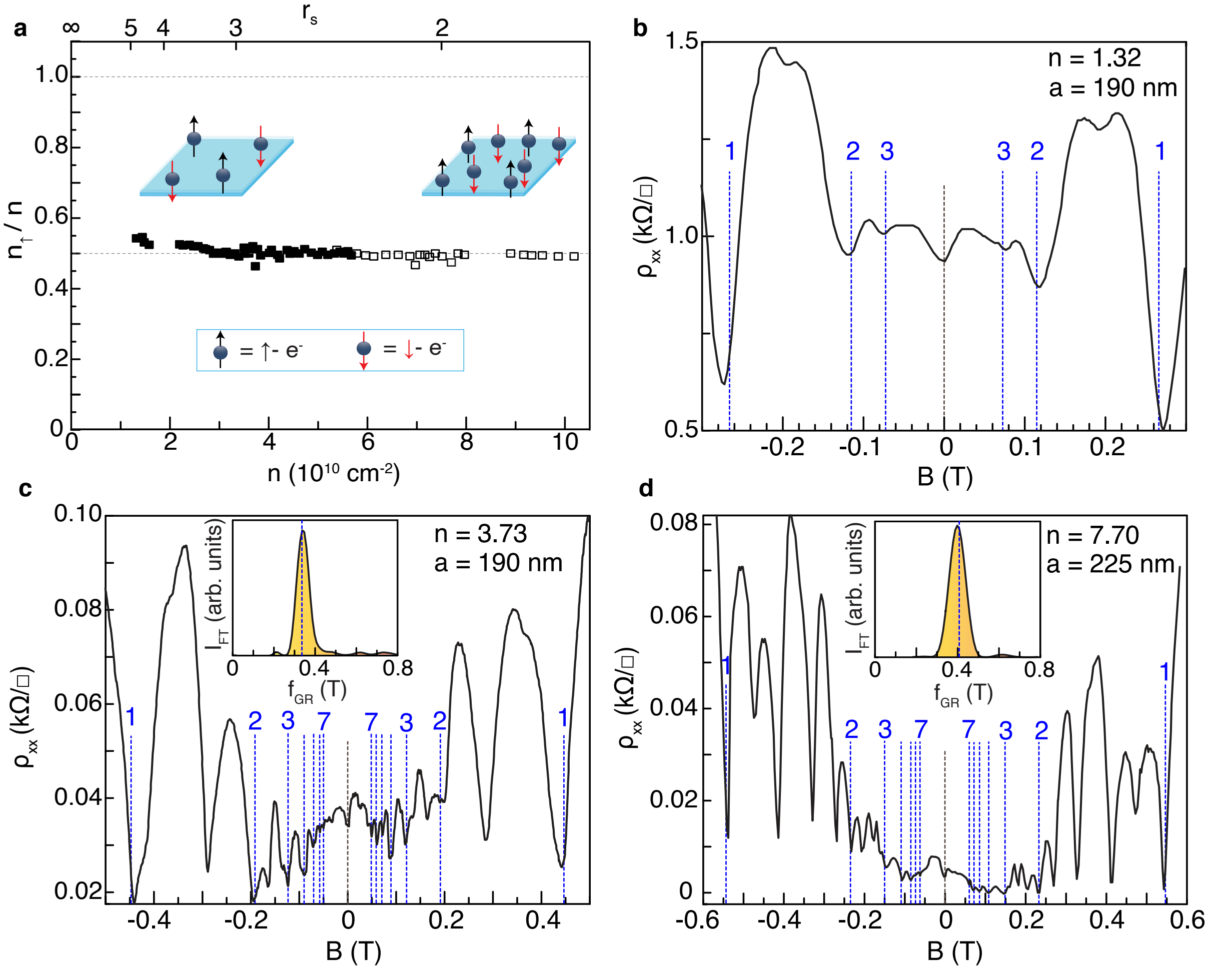


**Fig.** S5: Spin polarization of zero-field electrons obtained from GR data. **a**, The measured electron densities of a particular spin, normalized to $n$, plotted against $n$. Filled and open squares represent data from two samples from different wafers. The 2DES is spin unpolarized even at very low densities. **b–d**, Magneto-resistance traces for three different 2DES densities, revealing many GR features flanking the V-shaped minimum at $B = 0$. Vertical blue lines mark the expected field positions of GRs, assuming a spin-unpolarized Fermi contour with $k_F = (2\pi n)^{1/2}$. Insets: Normalized Fourier transform (FT) spectra of the GR oscillations shown in **c** and **d**, respectively. The vertical blue lines mark the expected $f_{GR}$ assuming spin-unpolarized Fermi contours.

$2R_c/a = i - 1/4$ $(i = 1, 2, 3, ...)$,[S18–S24] where $R_c$ is the real-space cyclotron radius, and $a$ is the period of the perturbation. The size of $R_c$ is directly related to the electron Fermi wavevector $k_F$ according to $R_c = \hbar k_F/eB$. The magneto-resistance traces of Fig. S5**b–d**, are representative of

such GRs, exhibiting pronounced resistance minima at $B_i = 2\hbar k_F/ea(i - 1/4)$.

In the case of very low densities such as $n = 1.32$, there are very few GR features and they are easy to track [Fig. S5b]. Therefore, we can deduce $k_F$ directly from the field positions of GRs. At higher densities, however, there is a large number of GR features thanks to the high mobility of our sample. Also, the field positions of the GR features overlap with the Shubnikov-de Haas oscillations and we obtain a superposition of these two sets of oscillations. Therefore, we perform a Fourier transform (FT) analysis to extract the frequency of GR oscillations [shown in the insets of Figs. S5**c–d**]. The frequency of the GR oscillations, $f_{GR} = 2\hbar k_F/ea$, directly yields $k_F$. Using the deduced $k_F$, we can obtain an estimate of the spin polarization according to $n_\uparrow/n = k_F/(4\pi n)^{1/2}$. The FT spectra for both $n = 3.73$ and 7.70 exhibit a single peak whose position is consistent with a circular, spin-unpolarized Fermi contour having $k_F = (2\pi n)^{1/2}$. To better show this match in Figs. S5**b–d**, vertical blue lines are placed which mark the expected GR positions for such a Fermi contour assuming $k_F = (2\pi n)^{1/2}$.

# V. Theory

In this Section we describe the details of theoretical calculations. We begin with the wavefunction of the CF Fermi sea state in the periodic torus geometry, followed by a brief outline of the fixed-phase diffusion Monte Carlo (DMC) method for treating the effect of LL mixing (LLM). The most direct method for determining the critical Zeeman energy (above which the system is fully spin-polarized) would be to begin with a fully-spin-polarized CF Fermi sea and calculate the gain in the energy when one CF is moved from the top of the Fermi sea to the bottom of the spin-reversed Fermi sea. This calculation, unfortunately, is not possible because of the significant finite-size effects arising from the deviation in the shape of the Fermi sea from a perfect circle. Fortunately, we find that the *change* in energy due to LLM is reasonably well behaved as a function of the number of particles $N$ for both the fully-spin-polarized and the spin-singlet CF

Fermi seas. Our strategy is therefore to calculate the change in the energies of the spin-polarized and spin-singlet CF Fermi seas as a function of $r_s$. We incorporate the Zeeman energy through the Stoner model, which assumes that CFs of opposite spins interact through a contact interaction. We determine the values of the parameters in the Stoner model that produce transitions at the experimentally observed densities, and find that these are in reasonable agreement with those obtained from the microscopic CF theory. We assume zero temperature below.

## V.1. Wavefunction of the composite fermion Fermi-sea state

We will employ the torus geometry which is most suitable for investigating the CF Fermi sea. In our calculations below we consider a square sample of side $L$ (in units of the magnetic length $l_B$) with periodic boundary conditions. The lowest-LL (LLL) wavefunction for the fully-spin-polarized CF Fermi sea in this geometry was introduced in Refs. *(S26–S29)*:

$$\Psi^{\rm CF}_{\nu=\frac{1}{2}} = {\rm P_{LLL}} \det\left[\exp\left({\rm i}\mathbf{k}_{\rm n}\cdot\mathbf{r}_{\rm m}\right)\right]\Psi_1^2. \tag{S1}$$

Here $\det\left[\exp\left({\rm i}\mathbf{k}_n\cdot\mathbf{r}_m\right)\right]$ is the Fermi sea of free fermions, $\Psi_1^2$ (defined below) attaches two quantized vortices to each electron to convert it into a CF, and ${\rm P_{LLL}}$ projects the wavefunction into the LLL. The allowed wavevectors are:

$$\mathbf{k} = n_1\mathbf{b}_1 + n_2\mathbf{b}_2 \quad (n_1 \text{ and } n_2 \text{ integers}) \tag{S2}$$

with

$$\mathbf{b}_1 = \left(\frac{2\pi}{L}, 0\right),\ \mathbf{b}_2 = \left(0, \frac{2\pi}{L}\right). \tag{S3}$$

The number of flux quanta penetrating the square is given by $N_\phi = L^2/2\pi$, which is quantized to be an integer. $\Psi_1$ is the wavefunction of the lowest filled LL in effective magnetic field $B^* = B/2$:

$$\Psi_1[z_i, \bar{z}_i] = e^{\sum_i \frac{z_i^2 - |z_i|^2}{8l_B^2}} R_1(Z) \prod_{i,j,i<j} \theta\left(\frac{z_i - z_j}{L}|\tau\right), \tag{S4}$$

with

$$R_1(Z) = e^{-i\frac{\pi N}{L}Z}\theta\left(\frac{Z}{L} - \frac{\pi N(\tau-1)}{2\pi}|\tau\right), \tag{S5}$$

where $z_j = x_j + iy_j$ denotes the coordinates of the $j$th electron as a complex number, $Z = \sum_{i=1}^{N} z_i$ is the center of mass coordinate, and $\theta$ is the odd Jacobi theta function:[S29]

$$\theta(z|\tau) = \sum_{n=-\infty}^{\infty} e^{i\pi\left(n+\frac{1}{2}\right)^2\tau} e^{i2\pi\left(n+\frac{1}{2}\right)\left(z+\frac{1}{2}\right)}. \tag{S6}$$

Here, we have $\tau = i$ for the square torus. The explicit wavefunction after projection into the lowest LL through the Jain-Kamilla method[S30–S32] is given by:

$$\Psi^{\rm CF}_{\nu=\frac{1}{2}} = e^{\sum_i \frac{z_i^2-|z_i|^2}{4l_B^2}}\left[R_1(Z + \mathrm{i}l_B^2\sum_j k_j)\right]^2 \det G_{k_n}(z_m) \tag{S7}$$

with

$$G_{k_n}(z_m) \;=\; e^{-\frac{k_n l_B^2}{4}\left(k_n+2\bar{k}_n\right)} e^{\frac{\mathrm{i}}{2}(\bar{k}_n+k_n)z_m} \times \prod_{j,j\neq m}\theta\left(\frac{z_m + \mathrm{i}2k_n l_B^2 - z_j}{L}|\tau\right). \tag{S8}$$

The wavefunction for the spin-singlet Fermi sea[S33] is obtained by making the replacement in Eq. S7:

$$\det G_{k_n}(z_m) \to \det{}_{\uparrow} G_n(z_m)\ \det{}_{\downarrow} G_n(z_m). \tag{S9}$$

Here $\det_{\uparrow} G_n(z_m)$ is the determinant of an $\frac{N}{2}\times\frac{N}{2}$ matrix corresponding to the $N/2$ spin-up electrons (with spatial coordinates from $z_1$ to $z_{N/2}$), and $\det_{\downarrow} G_n(z_m)$ is an analogous determinant for the remaining spin-down electrons.

The Coulomb interaction is given by:[S32, S34]

$$E = W + \frac{1}{N}\frac{2\pi}{L^2}\sum_{i<j}\sum_{\mathbf{q}\neq 0}\frac{1}{q}e^{i\mathbf{q}\cdot(\mathbf{r}_i-\mathbf{r}_j)} \tag{S10}$$

in units of $E_{\rm C}$. Here we have $\mathbf{q} = \left(\frac{2\pi m}{L}, \frac{2\pi n}{L}\right)$, where $m$ and $n$ are integers. The first term represents the self-interaction between electrons and their images, given by:[S35]

$$W = -\frac{1}{L}\left[2 - \sum_{m,n}{}' \varphi_{-1/2}(\pi(\tau m^2 + \tau^{-1}n^2))\right]$$
$$\varphi_n(z) \equiv \int_1^\infty dte^{-zt}t^n \ , \tag{S11}$$

where the prime on $\sum'$ indicates that the $m = n = 0$ term is to be excluded. The second term on the right hand side of Eq. S10 represents the electron-electron, electron-background and background-background interactions; the $\mathbf{q} = 0$ term is excluded because it is canceled by the sum of the electron-background and background-background interactions.

## V.2. Fixed-phase DMC method

The wavefunctions described above are confined to the LLL. To deal with the experimental phenomenon we need to estimate how these wavefunctions are modified by LLM. We will employ the fixed-phase DMC method for this purpose. The strength of LLM is conveniently characterized by the parameter $\kappa = E_C/\hbar\omega_c$, where $\hbar\omega_c = \hbar eB/m$ is the cyclotron energy. For $\nu = 1/2$ we have the relation $r_s = 2\kappa$, and we will depict our results as a function of $r_s$. For parameters of n-doped GaAs (electron band mass $m = 0.067m_e$, dielectric function $\varepsilon = 13$, and Landé g factor $g = -0.44$), $r_s$ is related to density as $n \approx (32.8/r_s^2) \times 10^{10}$ cm$^{-2}$.

The DMC method[S36,S37] can obtain the 'exact' ground-sate energy for certain interacting systems. The essential idea is that for wavefunctions that are real and non-negative, the Schrödinger equation in imaginary time:

$$-\hbar\partial_t\Psi\left(\mathbf{R},t\right) = \left[H\left(\mathbf{R}\right) - E_T\right]\Psi\left(\mathbf{R},t\right) \tag{S12}$$

and can be interpreted as a diffusion equation, with $\Psi\left(\mathbf{R},t\right)$ playing the role of the density distribution. Here $\mathbf{R} = (\mathbf{r}_1, \mathbf{r}_2, \ldots, \mathbf{r}_N)$ collectively denotes the positions of all particles and

$E_T$ is a constant energy offset introduced for the convenience of numerical computation. The Schrödinger equation may be written in terms of Green's function:

$$\Psi\left(\mathbf{R}, t+\tau\right) = \int G\left(\mathbf{R} \to \mathbf{R}', \tau\right) \Psi\left(\mathbf{R}, t\right) d\mathbf{R} \tag{S13}$$

where

$$G\left(\mathbf{R} \to \mathbf{R}', \tau\right) = \langle \mathbf{R}' | \exp\left[ -\frac{\tau\left(H\left(\mathbf{R}\right) - E_T\right)}{\hbar} \right] |\mathbf{R}\rangle. \tag{S14}$$

In the large imaginary-time limit the evolution operator projects out the ground state provided it has non-zero overlap with the initial trial wavefunction. DMC is a stochastic projector method for implementing the evolution in imaginary time through an importance sampling scheme using a trial or guiding wavefunction. In the absence of a potential, we have the distribution of random walkers (or diffusing Brownian particles) in the $2N$ dimensional configuration space. In the presence of a potential, the most effective method is through a branching (or a birth/death) algorithm in which either a walker dies with some probability in regions of high potential energy, or new walkers are created in regions of low potential energy, according to certain rules that have been discussed extensively in the literature.

The wavefunction of the CF Fermi sea is not real due to the broken time-reversal symmetry in the presence of a magnetic field. To circumvent this problem, we use the fixed-phase DMC method.[S38–S41] Here one expresses the wavefunction as:

$$\Psi = |\Psi| \exp\left[i\Phi\right]. \tag{S15}$$

Taking the phase $\Phi(\mathbf{R})$ to be fixed, the Schrödinger equation for the amplitude is given by:

$$H\left|\Psi\left(\mathbf{R}, t\right)\right| = \left( -\sum_{i=1}^{N} \frac{\hbar^2 \nabla_i^2}{2m} + V_{\text{eff}}\left(\mathbf{R}\right) - E_T \right) \left|\Psi\left(\mathbf{R}, t\right)\right| = E\left|\Psi\left(\mathbf{R}, t\right)\right|, \tag{S16}$$

where

$$V_{\text{eff}}\left(\mathbf{R}\right) = V\left(\mathbf{R}\right) + \frac{1}{2m} \sum_{i=1}^{N} \left[ \hbar \nabla_i \Phi\left(\mathbf{R}\right) + \frac{e}{c} \mathbf{A}\left(\mathbf{r}_i\right) \right]^2 \tag{S17}$$

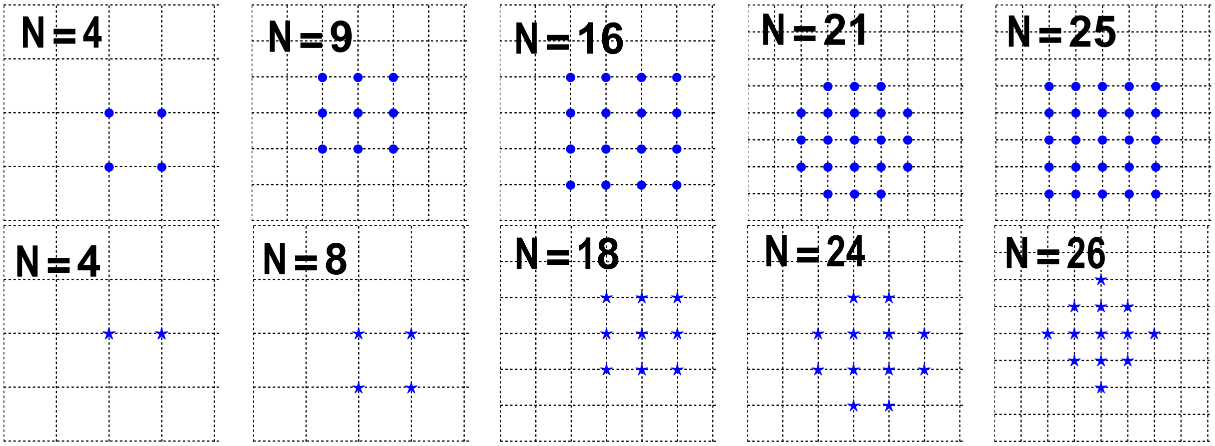


**Fig.** S6: Upper row: Momentum configurations of the fully-spin-polarized CF Fermi sea as a function of $N$, the number of CFs. The dots represent single particle momenta occupied by CFs (all with the same spin). Lower row: Momentum configurations of the spin-singlet CF Fermi sea. The stars mark momenta occupied by both spin-up and spin-down CFs.

is an effective interaction potential. Treating this with DMC now gives the lowest energy within the chosen phase sector, provided that $|\Psi(\mathbf{R}, t)|$ has a non-zero overlap with the lowest-energy state in that phase sector. The accuracy of the fixed-phase DMC depends on the choice of the phase (which is fixed using a trial wavefunction). Previous work has indicated[S40,S41] that the phase is not strongly affected by LLM, and hence it is a good starting point to fix the phase using the accurate LLL wave functions of the CF theory. That is the approach we follow.

## V.3. Calculation of $E_p$ and $E_s$

We find that the thermodynamic extrapolations of the energies $E_p(r_s)$ and $E_s(r_s)$ are not sufficiently accurate to capture the subtle physics of our interest, because of finite size deviations from circularity of the available Fermi seas in the torus geometry. We therefore write:

$$E_p(r_s) - E_s(r_s) = E_p(0) - E_s(0) + \Delta E_p(r_s) - \Delta E_s(r_s) \qquad \text{(S18)}$$

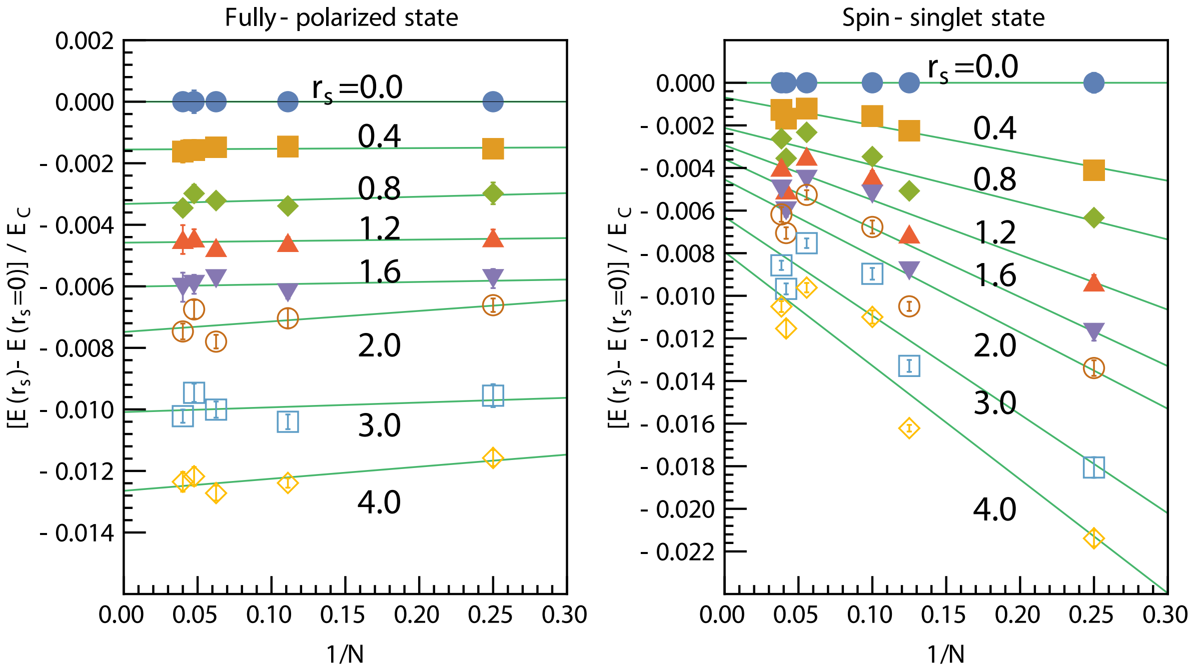


**Fig.** S7: Left Panel: The change in energy as a function of $r_s$ for the fully-polarized CF Fermi sea as a function of the number of particles $N$. The error arising from Monte Carlo sampling is shown for each point. The data points deviate from the regression line, indicating relative big errors in estimating the intercepts of the regression lines. However, the spacing between different regression lines is more or less uniform, implying that the slope of the $\Delta E_p$ vs. $r_s$ line has less uncertainty. Right Panel: Same as in the left panel, but for the spin-singlet CF Fermi sea.

where $\Delta E_p(r_s) = E_p(r_s) - E_p(r_s = 0)$ and $\Delta E_s(r_s) = E_s(r_s) - E_s(r_s = 0)$ are changes in the (per particle) energies of spin-polarized and spin-singlet Fermi sea states as a function of LLM. The quantities $\Delta E_p(r_s)$ and $\Delta E_s(r_s)$ are relatively well behaved as a function of $N$ and allow reasonable thermodynamic extrapolations.

The Fermi seas we have used to calculate $E_p(r_s)$ and $E_s(r_s)$ are shown in Fig. S6. To approximate the ground state, we have made the Fermi surface as compact and circular as possible within the finite-size constraints. Because of the computational complexity, we have reached systems containing up to 25 CFs for the fully-polarized state and 26 CFs for the spin-singlet state. The behavior of $E(r_s) - E(0)$ for fully-polarized and spin-singlet CF Fermi seas as

a function of $1/N$ is shown in Fig. S7. The thermodynamic limits of $E(r_s) - E(0)$ are obtained from linear regression, with the error defined as the standard deviation of the calculated values from the regressed values. The resulting $E(r_s) - E(0)$ are shown in the main text for both the spin-polarized and spin-singlet CF Fermi seas.

## V.4. Stoner model for composite fermions

For a direct comparison with the experiment it is necessary to incorporate the non-zero Zeeman energy. We shall do so within the Stoner model of itinerant magnetism. Given that the experimental phase transitions arise as a result of an extremely subtle competition between various energies, our strategy in this section will be to determine the parameters of the Stoner model that produce the experimental values of the critical densities where the two phase transitions are observed. We find that these values are generally consistent with those obtained directly from microscopic calculations.

We consider an effective Hubbard Hamiltonian for CFs:

$$\mathcal{H} = \sum_{k,\sigma} \left( E_k - \sigma \frac{E_Z}{2} \right) c^\dagger_{k\sigma} c_{k\sigma} + \frac{U}{n} \int d^2 r n_\uparrow(\mathbf{r}) n_\downarrow(\mathbf{r}). \tag{S19}$$

Here $E_k$ is the single-particle kinetic energy. The parameter $\sigma$ labels the spin with $\sigma = +1$ (or $\sigma = \uparrow$ ) and $\sigma = -1$ ($\sigma = \downarrow$ ) representing spin-up and spin-down. $E_Z$ is the Zeeman energy, defined as the energy required to flip a spin. It is assumed that the interaction is a contact interaction between spin-up and spin-down CFs, with its strength characterized by the parameter $U$. The quantity $n = N/A$ is the average areal density of the CFs where $N$ is the total number of CFs and $A$ is the total area. $N_\uparrow$ and $N_\downarrow$ are the number of spin-up and spin-down CFs, with $N = N_\uparrow + N_\downarrow$, and $n_\uparrow(\mathbf{r})$ and $n_\downarrow(\mathbf{r})$ are the local densities for spin-up and spin-down CFs. In a mean-field approximation, the above Hamiltonian simplifies to:

$$\mathcal{H} = \sum_{k,\sigma} E_k c^\dagger_{k\sigma} c_{k\sigma} - \frac{P E_Z N}{2} - \frac{P^2 U N}{4} + \frac{U N}{4}, \tag{S20}$$

where the polarization $P$ is defined as:

$$P = \frac{N_\uparrow - N_\downarrow}{N}. \tag{S21}$$

We define the Fermi energies for spin-up (spin-down) CFs to be $E_F^\uparrow$ ($E_F^\downarrow$). We will assume that CFs have a parabolic dispersion with an effective mass that is independent of the spin polarization. Then, $E_F^\uparrow + E_F^\downarrow \equiv E_F$ is a constant, equal to the Fermi energy of the fully-spin-polarized Fermi sea, and the density of states per unit area for each spin is given by $n/E_F$. The polarization can be expressed as:

$$P = \frac{E_F^\uparrow - E_F^\downarrow}{E_F} \tag{S22}$$

From Eq. S20, the ground state energy density is given by:

$$\frac{E}{A} = \frac{n(E_F - U)}{4}\left(P - \frac{E_Z}{E_F - U}\right)^2 - \frac{E_Z^2 n}{4(E_F - U)} + \frac{(U + E_F)n}{4}. \tag{S23}$$

The range of $P$ is $-1 \leq P \leq 1$, where $P = \pm 1$ represents the fully-spin-polarized state and $P = 0$ the spin-singlet state.

For $E_Z$=0, Eq. S23 yields:

$$E_p - E_s = \frac{E_F - U}{4} \tag{S24}$$

where $E_p$ and $E_s$ are the energies per particle for the fully-spin-polarized and spin-singlet states.

For $E_Z \neq 0$, the minimum total energy from Eq. S23 is obtained at $P = \frac{E_Z}{E_F - U}$. Of course, the polarization is restricted to $|P| \leq 1$, and a transition from a fully-spin-polarized state to a partially-spin-polarized state occurs for $P = 1$ (assuming $E_Z > 0$), which gives the critical Zeeman energy $E_Z^{\text{crit}} = E_F - U = 4(E_p - E_s)$. The transition from $|P| = 1$ to $|P| < 1$ thus occurs at:

$$E_Z = E_Z^{\text{crit}} = 4(E_p - E_s). \tag{S25}$$

Now, motivated by our DMC results which show that $E_p(r_s) - E_s(r_s)$ varies linearly with $r_s$ for small $r_s$, we model the right hand side of Eq. S25 as $E_p(r_s) - E_s(r_s) = [E_p(r_s =$

| | Eq. S26 fitted to experiment | microscopic calculation |
|---|---|---|
| $\gamma$ | 0.00088 | 0.0012(2) (this work) |
| $E_Z^{\rm crit}(0)/E_C$ | 0.020 | 0.022 [Ref.[S3]] |

**Table** S1: The second column gives the values of parameters of the Eq. S26 that produce transitions at the densities $n_{c1} = 3.5 \times 10^{10}$ cm$^{-2}$ and $n_{c2} = 4.2 \times 10^{10}$ cm$^{-2}$. The last column displays the values of these parameters obtained from microscopic calculations using either fixed-phase DMC method (this work), or variational Monte Carlo method.[S3] The microscopic calculations assume a purely 2D system.

$0) - E_s(r_s = 0)] - \gamma r_s E_C$. A polarization transition occurs at $E_Z$ given by:

$$\frac{E_Z}{E_C} = \frac{E_Z^{\rm crit}(r_s = 0)}{E_C} - 4\gamma r_s. \tag{S26}$$

Our DMC calculations give $\gamma = 0.0012(2)$. Taking $E_Z^{\rm crit}(r_s = 0)/E_C = 0.022$ from earlier calculation[S3] yields the phase diagram shown in the main text.

A slightly different, although closely related, analysis is as follows. Because $E_Z/E_C \propto 1/r_s$ and $E_Z^{\rm crit}(r_s = 0)/E_C$ is a constant, Eq. S26 is quadratic in $r_s$, and therefore may admit two real solutions for $r_s$ (or density). Table S1 shows the values of the parameters $E_Z^{\rm crit}(r_s = 0)/E_C$ and $\gamma$ that produce transitions at densities $n_{c1} = 3.5 \times 10^{10}$ cm$^{-2}$ and $n_{c2} = 4.2 \times 10^{10}$ cm$^{-2}$, where transitions are experimentally observed. The values of these parameters calculated directly from the microscopic CF theory are shown in the last column of Table S1. We find that the numbers given in the last two columns are in satisfactory agreement, especially in view of the crude nature of the Stoner model (which only accounts for the contact interaction between CFs of opposite spins and assumes that $U$ and the CF mass do not depend on the polarization), the various approximations made within the microscopic calculations (neglect of finite thickness; fixed-phase approximation), and the fact that the energy differences are only a fraction of 1% of the individual energies.

One may consider the situation where the Zeeman coupling is switched off entirely, as is possible, in principle, by application of hydrostatic pressure. In this case, the CF Fermi sea

is spin singlet for small $r_s$, but a Bloch transition occurs, according to Eq. S26, at $r_s \approx 4.6$. While the precise value of the critical $r_s$ depends on the accuracy of the approximations and assumptions, we believe that our calculations make a strong case for Bloch ferromagnetism for CFs at sufficiently low densities. These calculations also demonstrate that the Bloch transition for CFs occurs at relatively small values of $r_s \approx 4 - 5$ compared to the Bloch transition for electrons that is predicted for $r_s \approx 26$. At what $r_s$ the transition occurs is a complex function of the relative importance of the interaction and the kinetic energies, and a full quantum Monte Carlo calculation is required even for electrons. The interaction for composite fermions is much more complex than that between electrons. Some insight into why the Bloch transition occurs at smaller $r_s$ at $\nu = 1/2$ than that for the electrons at $B = 0$ can be gained from the observation that the CF mass is much smaller than the electron band mass, thereby diminishing the importance of the CF kinetic energy.

# VI. Related phenomena

## VI.1. Bloch ferromagnetism vis-à-vis the Mermin Wagner theorem in 2D electron systems

In a seminal paper in 1966, Mermin and Wagner (MW) proved that, at any non-zero temperature, there can be no ferromagnetism in one or two dimensions.[S42] The model MW use is the isotropic Heisenberg spin system with finite-range exchange interaction, and their conclusion is based on theoretically demonstrating that spin-fluctuations destabilize ferromagnetic (as well as anti-ferromagnetic) order in an infinitely-large system without a symmetry-breaking field. We would like to note that the MW theorem is not directly applicable to our experiments, because of both the finite sample size (about 100 $\mu$m by 50 $\mu$m) and the presence of a symmetry-breaking (magnetic) field. We also note that the theoretical calculations above have been performed for zero temperature, and thus deal only with the ground-state properties.

## VI.2. Spontaneous valley polarization in 2D systems with anisotropic effective mass

A recent theory by Zhu *et al.*[S43] predicts that in 2DESs where electrons occupy two valleys with a large effective mass anisotropy, for a sufficiently large anisotropy, the CF Fermi sea at $\nu = 1/2$ undergoes a transition to a valley-polarized ground state. The theory does not consider the role of density, $r_s$, or LLM, and the transition depends only on the mass anisotropy. 2DESs confined to AlAs quantum wells have the required large mass anisotropy, and some of the experimental piezo-resistance traces taken as a function of uniaxial, in-plane strain in AlAs 2DESs indeed give a hint of spontaneous valley polarization.[S43,S44] However, similar data taken on samples with better quality suggest otherwise.[S45,S46] We emphasize that it is not obvious whether there is any connection of this phenomenon to the Bloch ferromagnetism in the CF Fermi sea that we discuss in our work here. In particular, as stated above, the valley polarization considered in Ref.[S43] does not depend on the density or $r_s$ but the spin polarization we report here does.

## VI.3. Spin polarization of 2D electrons in monolayer $MoS_2$

During the writing of our manuscript, we became aware of very recent experiments by Roch $et$ $al.$[S47] on a 2DES in a monolayer of $MoS_2$. (We thank R. Warburton for bringing this work to our attention.) In $MoS_2$, $r_s$ is large thanks to the large electron effective mass and small dielectric constant. On the other hand, $MoS_2$ has a complex energy band structure: the 2D electrons occupy multiple conduction-band valleys and also there is a strong spin-orbit interaction, linking the spin and valley degrees of freedom. Roch *et al.* report the observation of spin-polarized electrons in a magnetic field of 9.0 T and at electron densities up to $n = 5 \times 10^{12}$ cm$^{-2}$, which corresponds to $r_s \simeq 5$. A subsequent theoretical work[S48] supports such a ferromagnetic phase. In this theory, the ferromagnetism arises from non-analyticities which go beyond Fermi liquid theory. It is also worth noting that magneto-transport data in nominally similar samples at

comparable densities and magnetic fields[S49] exhibit Shubnikov-de Haas oscillations which do not appear to be consistent with a fully-polarized system.

# References


S1. Jain, J. K. *Composite fermions*. (Cambridge University Press, New York, 2007).

S2. Liu, Y., Hasdemir, S., Wójs, A., Jain, J. K., Pfeiffer, L. N., West, K. W., Baldwin, K. W. & Shayegan, M. Spin polarization of composite fermions and particle-hole symmetry breaking. *Phys. Rev. B* **90**, 085301 (2014).

S3. Park, K. & Jain, J. K. Phase diagram of the spin polarization of composite fermions and a new effective mass. *Phys. Rev. Lett.* **80**, 4237 (1998).

S4. Kravchenko, S. V. & Sarachik, M. P. Metal-insulator transition in two-dimensional electron systems. *Rep. Prog. Phys.* **67**, 1 (2004).

S5. Spivak, B., Kravchenko, S. V., Kivelson, S. A. & Gao, X. P. A. Colloquium: Transport in strongly correlated two-dimensional electron fluids. *Rev. Mod. Phys.* **82**, 1743 (2010).

S6. Vakili, K., Shkolnikov, Y. P., Tutuc, E., De Poortere, E. P. & Shayegan, M. Spin susceptibility of two-dimensional electrons in narrow AlAs quantum wells. *Phys. Rev. Lett.* **92**, 226401 (2004).

S7. Li, S., Zhang, Q., Ghaemi, P., & Sarachik, M. P. Evidence for mixed phases and percolation at the metal-insulator transition in two dimensions. *Phys. Rev. B* **99**, 155302 (2019).

S8. Pudalov, V. M., Kutsevich, A. Y., Gershenson, M. E., Burmistrov, I. S. & Reznikov, M. Probing spin susceptibility of a correlated two-dimensional electron system by transport and magnetization measurements. *Phys. Rev. B* **98**, 155109 (2018).

S9. Zhu, J., Stormer, H. L., Pfeiffer, L. N., Baldwin, K. W. & West, K. W. Spin susceptibility of an ultra-low-density two-dimensional electron system. *Phys. Rev. Lett.* **90**, 056805 (2003).

S10. Dolgopolov, V. T. & Gold, A. Magnetoresistance of a two-dimensional electron gas in a parallel magnetic field. *JETP Lett.* **71**, 27 (2000).

S11. Herbut, I. F. The effect of parallel magnetic field on the Boltzmann conductivity and the Hall coefficient of a disordered two-dimensional Fermi liquid. *Phys. Rev. B* **63**, 113102 (2001).

S12. Li, Y. Q., Umansky, V., von Klitzing, K. & Smet, J. H. Nature of the spin transition in the half-filled Landau level. *Phys. Rev. Lett.* **102**, 046803 (2009).

S13. Padmanabhan, M., Gokmen, T. & Shayegan, M. Density dependence of valley polarization energy for composite fermions. *Phys. Rev. B* **80**, 035423 (2009).

S14. Melinte, S., Freytag, N., Horvatić, M., Berthier, C., Lévy, L. P., Bayot, V. & Shayegan, M. NMR determination of 2D electron spin polarization at $\nu = 1/2$. *Phys. Rev. Lett.* **84**, 354 (2000).

S15. Freytag, N., Horvatić, M., Berthier, C., Shayegan, M., & Lévy, L. P. NMR Investigation of How Free Composite Fermions Are at $\nu = 1/2$. *Phys. Rev. Lett.* **89**, 246804 (2002).

S16. Tanatar, B. & Ceperley, D. M. Ground state of the two-dimensional electron gas. *Phys. Rev. B* **39**, 5005 (1989).

S17. Attaccalite, C., Moroni, S., Gori-Giorgi, P. & Bachelet, G. B. Correlation energy and spin polarization in the 2D electron gas. *Phys. Rev. Lett.* **88**, 256601 (2002).

S18. D. Weiss, von Klitzing, K., Ploog, K. & G. Weimann, Magnetoresistance Oscillations in a Two-Dimensional Electron Gas Induced by a Submicrometer Periodic Potential. *Europhys. Lett.* 8, 179 (1989)

S19. Gerhardts, R. R., Weiss, D. & von Klitzing, K. Novel magnetoresistance oscillations in a periodically modulated two-dimensional electron gas. *Phys. Rev. Lett.* **62**, 1173 (1989).

S20. Winkler, R. W., Kotthaus, J. P. & Ploog, K. Landau band conductivity in a two-dimensional electron system modulated by an artificial one-dimensional superlattice potential. *Phys. Rev. Lett.* **62**, 1177 (1989).

S21. Beenakker, C. W. J. Guiding-center-drift resonance in a periodically modulated two-dimensional electron gas. *Phys. Rev. Lett.* **62**, 2020 (1989).

S22. Kamburov, D., Shayegan, M., Winkler, R., Pfeiffer, L. N., West, K. W. & Baldwin, K. W. Anisotropic Fermi contour of (001) GaAs holes in parallel magnetic fields. *Phys. Rev. B* **86**, 241302(R) (2012).

S23. Kamburov, D., Mueed, M. A., Shayegan, M., Pfeiffer, L. N., West, K. W., Baldwin, K. W., Lee, J. J. D. & Winkler, R. Anisotropic Fermi contour of (001) GaAs electrons in parallel magnetic fields. *Phys. Rev. B* **88**, 125435 (2013).

S24. Mueed, M. A., Kamburov, D., Shayegan, M., Pfeiffer, L. N., West, K. W., Baldwin, K. W. & Winkler, R. Splitting of the Fermi Contour of Quasi-2D Electrons in Parallel Magnetic Fields, Splitting of the Fermi Contour of Quasi-2D Electrons in Parallel Magnetic Fields. *Phys. Rev. Lett.* **114**, 236404 (2015).

S25. Shao, J., Kim, E. -A., Haldane, F. D. M. & Rezayi, E. H. Entanglement Entropy of the $\nu = 1/2$ Composite Fermion Non-Fermi Liquid State. *Phys. Rev. Lett.* **114**, 206402 (2015).

S26. Wang, J., Geraedts, S. D., Rezayi, E. H. & Haldane, F. D. M. Lattice Monte Carlo for quantum Hall states on a torus. *Phys. Rev. B* **99**, 125123 (2019).

S27. Geraedts, S. D., Wang, J., Rezayi, E. H. & Haldane F. D. M. Berry Phase and Model Wave Function in the Half-Filled Landau Level. *Phys. Rev. Lett.* **121**, 147202 (2018).

S28. Pu, S., Fremling, M. & Jain, J. K. Berry phase of the composite-fermion Fermi sea: Effect of Landau-level mixing. *Phys. Rev. B* **98**, 075304 (2018).

S29. Mumford, D. Tata Lectures on Theta Vols. I and II (Birkhäuser Boston, 2007). ISBN 9780817645779.

S30. Jain, J. K. & Kamilla, R. K. Composite Fermions in the Hilbert Space of the Lowest Electronic Landau Level. *Int. J. Mod. Phys. B* **11**, 2621 (1997).

S31. Jain, J. K. & Kamilla, R. K. Quantitative study of large composite-fermion systems. *Phys. Rev. B* **55**, R4895(R) (1997).

S32. Pu, S., Wu, Y.-H. & Jain, J. K. Composite fermions on a torus. *Phys. Rev. B* **96**, 195302 (2017).

S33. Wu, X. G., Dev, G. & Jain, J. K. Mixed-spin incompressible states in the fractional quantum Hall effect. *Phys. Rev. Lett.* **71**, 153 (1993).

S34. Yoshioka, D., Halperin, B. I. & Lee, P. A. Ground State of Two-Dimensional Electrons in Strong Magnetic Fields and $1/3$ Quantized Hall Effect. *Phys. Rev. Lett.* **50**, 1219 (1983).

S35. Bonsall, L. & Maradudin, A. A. Some static and dynamical properties of a two-dimensional Wigner crystal. *Phys. Rev. B* **15**, 1959 (1977).

S36. Reynolds, P. J. & Ceperley, D. M. Fixed-node quantum Monte Carlo for molecules. *J. Chem. Phys.* **77**, 5593 (1982),

S37. Foulkes, W. M. C., Mitas, L., Needs, R. J. & Rajagopal, G. Quantum Monte Carlo simulations of solids. *Rev. Mod. Phys.* **73**, 33 (2001),

S38. Ortiz, G., Ceperley, D. M. & Martin, R. M. New stochastic method for systems with broken time-reversal symmetry: 2D fermions in a magnetic field. *Phys. Rev. Lett.* **71** 2777 (1993).

S39. Melik-Alaverdian, V., Bonesteel, N. E. & Ortiz, G. Quantum Hall Fluids on the Haldane Sphere: A Diffusion Monte Carlo Study. *Phys. Rev. Lett.* **79**, 5286 (1997).

S40. Zhang, Y., Wójs, A. & Jain, J. K. Landau-level mixing and particle-hole symmetry breaking for spin transitions in the fractional quantum Hall effect. *Phys. Rev. Lett.* **117**, 116803 (2016).

S41. Güçlü, A. D. & Umrigar, C. J. Maximum-density droplet to lower-density droplet transition in quantum dots. *Phys. Rev. B* **72**, 045309 (2005).

S42. Mermin, N. D. & Wagner, H. Absence of Ferromagnetism or Antiferromagnetism in One- or Two-Dimensional Isotropic Heisenberg Models. *Phys. Rev. Lett.* **17**, 1133 (1966).

S43. Z. Zhu, Sheng, D. N., Fu, L. & Sodemann, I. Valley Stoner instability of the composite Fermi sea. *Phys. Rev. B* **98**, 155104 (2018).

S44. M. Padmanabhan, Gokmen, T. & Shayegan, M. Composite fermion valley polarization energies: Evidence for particle-hole asymmetry. *Phys. Rev. B* **81**, 113301 (2010).

S45. Padmanabhan, M. Composite Fermions With A Valley Degree Of Freedom, PhD thesis, Princeton University, 2010; page 55.

S46. Hossain, M. S., Ma, M. K., Pfeiffer, L. N., West, K. W., Baldwin, K. W. & Shayegan, M. unpublished.

S47. J. G. Roch, Froehlicher, G., Leisgang, N., Makk, P., Watanabe, K., Taniguchi, T. & Warburton, R. J. Spin-polarized electrons in monolayer $MoS_2$. *Nat. Nanotechnol.* **14**, 432–436 (2019).

S48. D. Miserev, Klinovaja, J. & Loss, D. Exchange intervalley scattering and magnetic phase diagram of transition metal dichalcogenide monolayers. *Phys. Rev. B* **100**, 014428 (2019).

S49. Pisoni, R., Kormànyos, A., Brooks, M., Lei, Z., Back, P., Eich, M., Overweg, H., Lee, Y., Rickhaus, P., Watanabe, K., Taniguchi, T., Imamoglu, A., Burkard, G., Ihn, T. & Ensslin, K. Interactions and Magnetotransport through Spin-Valley Coupled Landau Levels in Monolayer $MoS_2$. *Phys. Rev. Lett.* **121**, 247701 (2018).
